# Supplementary material for: Wide-Depth-Range 6D Object Pose Estimation in Space
Source: arXiv:2104.00337 source file (2021-04-01)
Supplement: Supplementary file 1 [file 6_appendix.tex]

% !TEX root = ../supp.tex
% !TEX spellcheck = en-US

\section{Physical Rendering of SwissCube}
\label{sec:appendix}

Although the European Space Agency has organized a satellite pose estimation challenge and released the SPEED satellite dataset, the unavailability of the target 3D model makes the pose accuracy not depending on the pose estimation method alone. Furthermore, the limited varieties of lighting also make it soon saturated and less discriminative, as discussed in Section~\ref{sec:related}.

To fully demonstrate the effectiveness of our method in space, we introduce the Swisscube satellite dataset. Swisscube is a Cubesat-type satellite which was designed at EPFL and launched in 2009. Given the accurate CAD files and material properties of each component of it, we synthesize photorealistic images using physically based rendering~\cite{xx}.

% !TEX root = ../top.tex
% !TEX spellcheck = en-US

\begin{table}
    \centering
    \begin{small}
    % \rowcolors{2}{white}{gray!10}
    \begin{tabular}{lcc}
        \toprule
        &	SPEED & {\bf CubeSat}\\
        \midrule
        % Synthetic  &12k & 40k \\
        % Real       & 5 & 300 \\
        % \midrule
        Size & 12k & 40k \\
        Accurate 3D model   &\xmark  & \cmark  \\
        Complex lighting    &\xmark  & \cmark \\
        Physical modeling    &\xmark  & \cmark \\
        Colors        &\xmark  & \cmark \\
        Sequences         &\xmark  & \cmark  \\
        Depth distribution & non-uniform & uniform \\
        \bottomrule
    \end{tabular}
    \end{small}
    % \vspace{-3mm}
    \caption{{\bf CubeSat dataset.} bla bla bla bla bla bla bla bla bla bla bla bla bla bla bla bla bla bla bla bla bla bla bla bla bla bla bla bla bla bla bla bla bla bla bla bla bla bla bla bla bla bla bla bla bla bla bla bla bla bla bla bla bla bla bla bla bla bla bla bla bla bla bla bla bla bla bla bla bla bla bla bla bla bla bla bla bla bla bla bla }
    \label{tab:swisscube_vs_speed}
\end{table} 

% -----------------------------------
% Physically-based spectral rendering

\subsubsection{Physically-based spectral rendering}

In this section we provide a high-level description of the Swisscube satellite dataset which collects 40'000  physically-based synthetic images. While the SPEED satellite dataset images were produced using an OpenGL-based RGB rendering framework, we opted for a physically-based approach, where every element of the rendering pipeline were carefully modeled to mimic reality.

While the RGB model is often used to render color images, using tristimulus RGB colors in the rendering simulation generally yields non-physical results. For instance, surface reflectance properties of an object can be highly dependent on the wavelengths, which won't be accurately reproduced with RGB values. In a spectral renderer, colors are represented as spectral power distributions, resulting in improved accuracy especially when measured spectral data is available. For the Swisscube dataset, using a spectral renderer was a necessity as it was a requirement to correctly model the spectral responses of the solar irradiance emission, material reflectance properties and Earth surface radiance. Although the rendering simulation uses spectral colors, the resulting images will be converted to RGB images.

Relying on a physically-based rendering pipeline also gives us more control on the dynamic range of the output images. Thus we were able to accurately reproduce highlights orders of magnitude brighter than darker region of the images. An appropriate gamma curve could then be applied to produce images that can be viewed on regular displays.

To achieve all of this, we build our pipeline around the Mitsuba 2 renderer [???] which is a highly modular open-source framework that supports spectral rendering.

% -------------------
% The 3D / CAD model

\subsubsection{Accurate 3D model from CAD data}

For this dataset, we modelled every mechanical parts of the SwissCube, such as solar panels, antennas, and screws based directly on the raw CAD files. We carefully assign material reflection properties to each part. Given the physically-based nature of the pipeline, it would be possible to use efficient material acquisition technique such as [???] in the future for better results. Due to confidential reasons, we only release the mesh geometry data of the combined SwissCube without separable pieces to the public, which is enough for perfect registration.

% Citation for material acquistion technique: https://rgl.epfl.ch/publications/Dupuy2018Adaptive

% --------------------
% Physically-based Sun

\subsubsection{Modeling a physically-based Sun emitter}

In order to correctly model the illumination from the Sun, we leveraged the vast literature in astrophysics. As the target object will be placed above the Earth atmosphere, it is not enough to use specular solar irradiance measurements made at ground surface [???] as those will be be affected by the highly variable and absorbing constituents of the Earth atmosphere. Instead, we rely on the air mass zero reference spectrum [???], also known as extraterrestrial solar irradiance, mainly based on data from satellites and space shuttle missions. Figure \ref{fig:swisscube_sun_spectrum} show its spectral power distribution. We then use a point light source to represent the Sun, placed at the correct distance to the Earth. Note that is was necessary to scale the Sun irradiance to account for its surface area.

% Groud surface citation: https://www.osapublishing.org/ao/abstract.cfm?uri=ao-21-3-554
% ASTM Standard Extraterrestrial Spectrum Reference: https://www.nrel.gov/grid/solar-resource/spectra-astm-e490.html

% !TEX root = ../top.tex
% !TEX spellcheck = en-US

\begin{figure}[t]
    \begin{center}
    \includegraphics[width=1.0\linewidth]{./fig/swisscube_sun_spectrum/sun_spectrum_plot.jpeg}
    % \fbox{\rule{0pt}{2in} \rule{0.25\linewidth}{0pt}}
    \end{center}
    \vspace{-6mm}
    \caption{{\bf Air mass zero solar spectral power distribution.} 
    }
    \label{fig:swisscube_sun_spectrum}
\end{figure}

% ---------------------------
% Modeling the stars / galaxy

\subsubsection{Modeling the stars and galaxies}

We also added galaxies and other astronomical objects to our pipeline as we believe those could distract the learning algorithm. Based on the HYG database star catalogue [???], we could generate a high-resolution environment map that we later used as an second emitter. The HYG database contains around 220 thousands astronomical objects, mostly galaxies but also star clusters and Nebulae along with information regarding their position and brightness. Figure \ref{fig:swisscube_stars_envmap} shows the astronomical object projected on a spherical coordinate 2D map with their respective physically-based brightness.

Compared to the sun illumination, the irradiance coming from the stars is orders of magnitude lower. On the other hand, to maximize the diversities of the generated data, we decided to increase the actual brightness of each star in the galaxies to make them more apparent in rendering, which we think is a beneficial perturbation for a dataset.

% !TEX root = ../top.tex
% !TEX spellcheck = en-US

\begin{figure}[t]
    \begin{center}
    \includegraphics[width=1.0\linewidth]{./fig/swisscube_stars_envmap/stars_envmap.jpeg}
    % \fbox{\rule{0pt}{2in} \rule{0.25\linewidth}{0pt}}
    \end{center}
    \vspace{-6mm}
    \caption{{\bf Astronomical objects environment map based on the HYG dataset.} 
    }
    \label{fig:swisscube_stars_envmap}
\end{figure}

% HYG database link: http://www.astronexus.com/hyg

% ---------------------------------------------------
% Modeling the Earth radiance using the VIIRS dataset

\subsubsection{Spectral Earth radiance using the VIIRS dataset}

Properly modeling the Earth is very important here as it often occupies a large portion of the images. Moreover, the Sun light reflecting off the Earth is drastically affecting the illumination of the target object. In our pipeline, the Earth is a represented as a very large sphere, reflecting light coming from the Sun emitter onto the target object or directly towards the camera. Based on the NASA Visible Infrared Imaging Radiometer Suite (VIIRS) Level-1B data products [????], we generated a spectral radiance texture to model the reflectance of the Earth and its atmosphere. The VIIRS data products are produced by whiskbroom scanning radiometers on satellites orbiting around the Earth at a nominal altitude of 829 km, providing a full daily coverage of the Earth. These data products include 6 bands in the visible spectrum with high spatial resolution which we could use to generate a spectral reflectance texture. Figure \ref{fig:swisscube_earth_renders} shows the result of this process compared to the use of a simple Earth albedo texture available from the NASA website [????].

% !TEX root = ../supp.tex
% !TEX spellcheck = en-US

\begin{figure}[t]
    \centering
    \begin{tabular}{ccc}
    \includegraphics[height=2.4cm]{fig/swisscube_earth_renders_L1/earth_L1_albedo_texture.png}&
    \includegraphics[height=2.4cm]{fig/swisscube_earth_renders_L1/earth_L1_spectral_texture.png}&
    \includegraphics[height=2.4cm]{fig/swisscube_earth_renders_L1/earth_L1_DSCOVR.png}\\
    (a)&(b)&(c)\\
    \end{tabular}
    \vspace{-3mm}
    \caption{\small {\bf Rendered Earth compared to DSCOVR photograph.} (a) Ground-level albedo texture doesn't account for the scattering effects introduced by the atmosphere, resulting in over saturated colors when viewed from space. (b) Rendering of the Earth using our spectral texture based on the VIIRS data products. (c) Ground-truth real photograph taken by the DSCOVR satellite at the L1 Lagrange point.}
    \label{fig:swisscube_earth_renders}
\end{figure}

% VIIRS website: https://earthdata.nasa.gov/earth-observation-data/near-real-time/download-nrt-data/viirs-nrt#ed-corrected-reflectance
% Earth albedo texture: https://visibleearth.nasa.gov/images/57735/the-blue-marble-land-surface-ocean-color-sea-ice-and-clouds/57737l
% Real image DSCOVR website: https://www.nesdis.noaa.gov/content/dscovr-deep-space-climate-observatory

\subsubsection{Bring everything together at real scale}

We placed all those elements in a virtual scene at the real scale to ensure high fidelity images and produce a more comprehensive dataset. We could then generate sequences of images, simulating various docking procedures by varying camera and target vehicle poses and respective speed. Each sequence contains 100 consecutive images.

To achieve highest reflection of the real world, we place the SwissCube in the actual-working orbits about 700 km above the Earth's surface during rendering and model most of the space-borne items, such as the Sun, the Earth, and galaxies, physically. 

Depth range.

\subsubsection{Dataset generation and specs}

We generate 400 sequences in total, each sequence contains 100 consecutive images with random angular speed between 0.xx to 0.xx.

Fig.~\ref{fig:swisscube_vs_speed} shows some examples of the generated SwissCube dataset.

bla bla bla bla bla bla bla bla bla bla bla bla bla bla bla bla bla bla bla bla bla bla bla bla bla bla bla bla bla bla bla bla bla bla bla bla bla bla bla bla bla bla 

As discussed Section~\ref{sec:related}. Table~\ref{tab:swisscube_vs_speed} shows the comparison between SwissCube and SPEED dataset. Note that, in SPEED dataset, there are 2998 more synthetic images and also 300 more real images in the test set. However, Their ground truth labels are not accessible, so here we do not take them into account.

\YH{TODO}

From the total 400 sequences of images in the SwissCube dataset, we take all the images from the first 300 sequences as our training set and that from the last 100 as the test. In this subsection, we will evaluate the methods' performance in different depth ranges, that is, the whole depth range will be divided to three regions denoted as {\it Near}, {\it Medium} and {\it Far}, which correspond to depth range [1d-4d], [4d-7d] and [7d-10d], respectively.
